# Supplementary material for: Pillar-0: A New Frontier for Radiology Foundation Models
Source: arXiv:2511.17803 source file (2025-11-21)
Supplement: Supplementary file 1 [file appendix.tex]

Appendix
